# Supplementary material for: Generalized relation between electromechanical responses at fixed voltage and fixed electric field
Source: arXiv:2206.13552 source file (2022-10-25)
Supplement: Supplementary file 1 [file SI.pdf]

# SUPPLEMENTARY INFORMATION
# Generalized relation between electromechanical responses at fixed voltage and fixed electric field

Daniel Bennett,[1,*] Daniel Tanner,[1,2] Philippe Ghosez,[1] Pierre-Eymeric Janolin,[2] and Eric Bousquet[1]

[1]*Physique Théorique des Matériaux, QMAT, CESAM, University of Liège, B-4000 Sart-Tilman, Belgium*

[2]*Université Paris-Saclay, CNRS, CentraleSupélec, Laboratoire SPMS, 91190 Gif-sur-Yvette, France*

(Dated: October 5, 2022)

## I. DERIVATIONS OF FIXED FIELD - FIXED VOLTAGE RELATIONS

### A. Piezoelectricity

The proper piezoelectric tensor, measured at fixed voltage drop, is

$$e_{\alpha\beta\gamma} \equiv -\left.\frac{\partial^2 \mathcal{F}'_\Omega}{\partial \mathcal{E}'_\alpha \partial \tilde{\eta}_{\beta\gamma}}\right|_{\{\tilde{\eta},\mathcal{E}'\}=0} = \frac{\partial P'_\alpha}{\partial \tilde{\eta}_{\beta\gamma}} , \tag{1}$$

where the reduced electric field variables are

$$\begin{aligned} \mathcal{E}' &= (I+\tilde{\eta})\,\mathcal{E} \\ P' &= \frac{\Omega}{\Omega_0}\,(I+\tilde{\eta})^{-1} P \\ D' &= \frac{\Omega}{\Omega_0}\,(I+\tilde{\eta})^{-1} D \end{aligned} , \tag{2}$$

as in the main text. The volume of the system is

$$\Omega = (I+\det(\tilde{\eta}))\,\Omega_0 , \tag{3}$$

which for infinitesimal strains is

$$\Omega = (1+\mathrm{tr}(\tilde{\eta}))\,\Omega_0 + \mathcal{O}(\tilde{\eta}^2) . \tag{4}$$

We would like to write Eq. (1) in terms of the improper tensor, measured at fixed electric field:

$$e^{(\mathrm{i})}_{\alpha\beta\gamma} \equiv -\left.\frac{\partial^2 \mathcal{F}_{\Omega_0}}{\partial \mathcal{E}_\alpha \tilde{\eta}_{\beta\gamma}}\right|_{\{\tilde{\eta},\mathcal{E}\}=0} = \frac{\partial P_\alpha}{\partial \tilde{\eta}_{\beta\gamma}} . \tag{5}$$

First, we write the reduced polarization $P'$ in terms of $P$:

$$P'_\alpha = \det(I+\tilde{\eta})\,(I+\tilde{\eta})^{-1}_{\alpha x} P_x , \tag{6}$$

where summation is assumed, using Latin letters for dummy indices and Greek letters for free indices. Eq. (6) can be further simplified using $\det(I+\tilde{\eta}) = 1+\mathrm{tr}(\tilde{\eta})+\mathcal{O}(\tilde{\eta}^2)$ and by expanding the $(I+\tilde{\eta})^{-1}$ term, assuming infinitesimal strain:

$$(I+\tilde{\eta})^{-1} = I-\tilde{\eta}+\tilde{\eta}^2-\tilde{\eta}^3+\dots , \tag{7}$$

which can easily be verified by multiplying both sides by $(I+\tilde{\eta})$. Note that it is important to make this approximation *before* differentiating. If we make the approximation after differentiating, we will retain contributions which are quadratic in strain.

* dbennett@uliege.be

Inserting Eq. (6) into Eq. (1) and differentiating, we get

$$\begin{aligned} e_{\alpha\beta\gamma} &= \frac{\partial\left((1+\tilde{\eta}_{ii})\left(\delta_{\alpha x}-\tilde{\eta}_{\alpha x}\right)P_x\right)}{\partial\tilde{\eta}_{\beta\gamma}} \\ &= \frac{\partial\left(P_\alpha+\tilde{\eta}_{ii}P_\alpha-\tilde{\eta}_{\alpha x}P_x+\mathcal{O}(\tilde{\eta}^2)\right)}{\partial\tilde{\eta}_{\beta\gamma}} \\ &= \frac{\partial P_\alpha}{\partial\tilde{\eta}_{\beta\gamma}}+\delta_{\beta\gamma}P_\alpha-\delta_{\alpha\beta}P_\gamma+\tilde{\eta}_{ii}\frac{\partial P_\alpha}{\partial\tilde{\eta}_{\beta\gamma}}-\tilde{\eta}_{\alpha x}\frac{\partial P_x}{\partial\tilde{\eta}_{\beta\gamma}} \\ &= e^{(\mathrm{i})}_{\alpha\beta\gamma}+\delta_{\beta\gamma}P_\alpha-\delta_{\alpha\beta}P_\gamma+\tilde{\eta}_{ii}\frac{\partial P_\alpha}{\partial\tilde{\eta}_{\beta\gamma}}-\tilde{\eta}_{\alpha x}\frac{\partial P_x}{\partial\tilde{\eta}_{\beta\gamma}} \end{aligned} . \tag{8}$$

The last two terms in the final two lines are proportional to $\tilde{\eta}$, which vanish since Eq. (1) is defined about $\tilde{\eta}\to 0$. Thus, we obtain the relation:

$$e_{\alpha\beta\gamma}=e^{(\mathrm{i})}_{\alpha\beta\gamma}+\delta_{\beta\gamma}P_\alpha-\delta_{\alpha\beta}P_\gamma\,. \tag{9}$$

### B. Electrostriction

The proper piezoelectric tensor, measured at fixed voltage drop, is

$$m_{\alpha\beta\gamma\delta}\equiv-\frac{1}{2}\left.\frac{\partial^3\mathcal{F}'_\Omega}{\partial\mathcal{E}'_\alpha\partial\mathcal{E}'_\beta\partial\tilde{\eta}_{\gamma\delta}}\right|_{\{\tilde{\eta},\mathcal{E}'\}=0}=\frac{\partial\varepsilon_{\alpha\beta}}{\partial\tilde{\eta}_{\gamma\delta}}\,. \tag{10}$$

As before, we would like to write this in terms of the improper electrostrictive tensor, measured at fixed electric field:

$$m^{(\mathrm{i})}_{\alpha\beta\gamma\delta}\equiv-\frac{1}{2}\left.\frac{\partial^3\mathcal{F}_{\Omega_0}}{\partial\mathcal{E}_\alpha\partial\mathcal{E}_\beta\partial\tilde{\eta}_{\gamma\delta}}\right|_{\{\tilde{\eta},\mathcal{E}\}=0}=\frac{\partial\varepsilon^{(\mathrm{i})}_{\alpha\beta}}{\partial\tilde{\eta}_{\gamma\delta}}\,, \tag{11}$$

where $\varepsilon^{(\mathrm{i})}_{\alpha\beta}\equiv\frac{\partial D_\alpha}{\partial\mathcal{E}_\beta}$ is the improper permittivity tensor, measured at fixed electric field calculated about the equilibrium state. Similarly to the case of piezoelectricity, we must write the proper permittivity in terms of the improper permittivity. Using the chain rule, we have

$$\varepsilon_{\alpha\beta}=\frac{\partial P'_\alpha}{\partial\mathcal{E}'_\beta}=\frac{\partial P'_\alpha}{\partial\mathcal{E}_y}\frac{\partial\mathcal{E}_y}{\partial\mathcal{E}'_\beta}\,. \tag{12}$$

Writing $\mathcal{E}$ in terms of $\mathcal{E}'$,

$$\begin{aligned} \mathcal{E}_y &= (I+\tilde{\eta})^{-1}{}_{yx}\mathcal{E}'_x \\ \implies \frac{\partial\mathcal{E}_y}{\partial\mathcal{E}'_\beta} &= (I+\tilde{\eta})^{-1}{}_{y\beta} \end{aligned} , \tag{13}$$

we get

$$\begin{aligned} \varepsilon_{\alpha\beta} &= (I+\tilde{\eta})^{-1}{}_{y\beta}\frac{\partial P'_\alpha}{\partial\mathcal{E}_y} \\ &= \det(I+\tilde{\eta})(I+\tilde{\eta})^{-1}{}_{\alpha x}(I+\tilde{\eta})^{-1}{}_{y\beta}\frac{\partial P_x}{\partial\mathcal{E}_y} \\ &= \det(I+\tilde{\eta})(I+\tilde{\eta})^{-1}{}_{\alpha x}(I+\tilde{\eta})^{-1}{}_{y\beta}\varepsilon^{(\mathrm{i})}_{xy} \end{aligned} , \tag{14}$$

which is exact, and can be further simplified for the case of infinitesimal strain:

$$\begin{aligned} \varepsilon_{\alpha\beta} &= (1+\tilde{\eta}_{ii})\left(\delta_{\alpha x}-\tilde{\eta}_{\alpha x}\right)\left(\delta_{y\beta}-\tilde{\eta}_{y\beta}\right)\varepsilon^{(\mathrm{i})}_{xy} \\ &= \left((1+\tilde{\eta}_{ii})\delta_{\alpha x}\delta_{y\beta}-\delta_{\alpha x}\tilde{\eta}_{y\beta}-\delta_{y\beta}\tilde{\eta}_{\alpha x}\right)\varepsilon^{(\mathrm{i})}_{xy}+\mathcal{O}(\tilde{\eta}^2) \\ &= (1+\tilde{\eta}_{ii})\varepsilon^{(\mathrm{i})}_{\alpha\beta}-\varepsilon^{(\mathrm{i})}_{\alpha y}\tilde{\eta}_{y\beta}-\tilde{\eta}_{\alpha x}\varepsilon^{(\mathrm{i})}_{x\beta}+\mathcal{O}(\tilde{\eta}^2) \end{aligned} . \tag{15}$$

So we get the following relation between proper and improper susceptibility tensors:

$$\varepsilon_{\alpha\beta} = (1+\tilde{\eta}_{ii})\varepsilon^{(\mathrm{i})}_{\alpha\beta} - \varepsilon^{(\mathrm{i})}_{\alpha i}\tilde{\eta}_{i\beta} - \tilde{\eta}_{\alpha j}\varepsilon^{(\mathrm{i})}_{j\beta} + \mathcal{O}(\tilde{\eta}^2)\,. \tag{16}$$

Note that $\varepsilon_{\alpha\beta} = \varepsilon^{(\mathrm{i})}_{\alpha\beta}$ at $\tilde{\eta} = 0$, which is expected. However, the terms proportional to $\tilde{\eta}$ must be retained as they will contribute to the strain derivative of the permittivity. Inserting Eq. (16) into Eq. (10):

$$\begin{aligned} m_{\alpha\beta\gamma\delta} &= \frac{\partial \varepsilon_{\alpha\beta}}{\partial \tilde{\eta}_{\gamma\delta}} \\ &= \frac{\partial}{\partial \tilde{\eta}_{\gamma\delta}}\left[(1+\tilde{\eta}_{ii})\varepsilon^{(\mathrm{i})}_{\alpha\beta} - \varepsilon^{(\mathrm{i})}_{\alpha i}\tilde{\eta}_{i\beta} - \tilde{\eta}_{\alpha j}\varepsilon^{(\mathrm{i})}_{j\beta} + \mathcal{O}(\tilde{\eta}^2)\right] \\ &= (1+\tilde{\eta}_{ii})\frac{\partial \varepsilon^{(\mathrm{i})}_{\alpha\beta}}{\partial \tilde{\eta}_{\gamma\delta}} + \varepsilon^{(\mathrm{i})}_{\alpha\beta}\delta_{\gamma\delta} - \frac{\partial \varepsilon^{(\mathrm{i})}_{\alpha i}}{\partial \tilde{\eta}_{\gamma\delta}}\tilde{\eta}_{i\beta} - \varepsilon^{(\mathrm{i})}_{\alpha i}\delta_{i\gamma}\delta_{\beta\delta} - \frac{\partial \varepsilon^{(\mathrm{i})}_{j\beta}}{\partial \tilde{\eta}_{\gamma\delta}}\tilde{\eta}_{\alpha j} - \varepsilon^{(\mathrm{i})}_{j\beta}\delta_{\alpha\gamma}\delta_{j\delta} \\ &= (1+\tilde{\eta}_{ii})\frac{\partial \varepsilon^{(\mathrm{i})}_{\alpha\beta}}{\partial \tilde{\eta}_{\gamma\delta}} + \varepsilon^{(\mathrm{i})}_{\alpha\beta}\delta_{\gamma\delta} - \varepsilon^{(\mathrm{i})}_{\alpha\gamma}\delta_{\beta\delta} - \varepsilon^{(\mathrm{i})}_{\delta\beta}\delta_{\alpha\gamma} - \frac{\partial \varepsilon^{(\mathrm{i})}_{\alpha i}}{\partial \tilde{\eta}_{\gamma\delta}}\tilde{\eta}_{i\beta} - \frac{\partial \varepsilon^{(\mathrm{i})}_{j\beta}}{\partial \tilde{\eta}_{\gamma\delta}}\tilde{\eta}_{\alpha j} \end{aligned} \,. \tag{17}$$

Setting $\tilde{\eta} \to 0$ after differentiating, we obtain

$$m_{\alpha\beta\gamma\delta} = m^{(\mathrm{i})}_{\alpha\beta\gamma\delta} + \varepsilon_{\alpha\beta}\delta_{\gamma\delta} - \varepsilon_{\alpha\gamma}\delta_{\beta\delta} - \varepsilon_{\delta\beta}\delta_{\gamma\alpha}\,. \tag{18}$$

### C. General

The proper response $A$, measured at fixed voltage drop, is

$$\begin{aligned} A_{\mathcal{E}_1\ldots\mathcal{E}_n\tilde{\eta}_1\tilde{\eta}_2} &\equiv -\frac{1}{n!}\left.\frac{\partial^n \mathcal{F}'_\Omega}{\partial \mathcal{E}'_{\mathcal{E}_1}\ldots\partial \mathcal{E}'_{\mathcal{E}_n}\partial \tilde{\eta}_{\tilde{\eta}_1\tilde{\eta}_2}}\right|_{\{\tilde{\eta},\mathcal{E}'\}=0}, \\ &= \frac{\partial \chi_{\mathcal{E}_1\ldots\mathcal{E}_n}}{\partial \tilde{\eta}_{\tilde{\eta}_1\tilde{\eta}_2}} \end{aligned} \tag{19}$$

where the proper $n^{\mathrm{th}}$ order susceptibility is defined as

$$\chi_{\mathcal{E}_1\ldots\mathcal{E}_n} \equiv \begin{cases} P'_{\mathcal{E}_1}, & n=1 \\ \frac{\partial D'_{\mathcal{E}_1}}{\partial \mathcal{E}'_{\mathcal{E}_2}}, & n=2 \\ \frac{\partial^{n-1} P'_{\mathcal{E}_1}}{\partial \mathcal{E}'_{\mathcal{E}_2}\ldots\partial \mathcal{E}'_{\mathcal{E}_n}}, & n>2 \end{cases}\,. \tag{20}$$

For $n = 1,2$, Eq. (20) is defined to be the polarization and permittivity, respectively. As before, we would like to write Eq. (19) in terms of the improper response, measured at fixed electric field:

$$\begin{aligned} A^{(\mathrm{i})}_{\mathcal{E}_1\ldots\mathcal{E}_n\tilde{\eta}_1\tilde{\eta}_2} &\equiv -\frac{1}{n!}\left.\frac{\partial^{n+1} \mathcal{F}_{\Omega_0}}{\partial \mathcal{E}_{\mathcal{E}_1}\ldots\partial \mathcal{E}_{\mathcal{E}_n}\partial \tilde{\eta}_{\tilde{\eta}_1\tilde{\eta}_2}}\right|_{\{\tilde{\eta},\mathcal{E}\}=0} \\ &= \frac{\partial \chi^{(\mathrm{i})}_{\mathcal{E}_1\ldots\mathcal{E}_n}}{\partial \tilde{\eta}_{\tilde{\eta}_1\tilde{\eta}_2}} \end{aligned}\,, \tag{21}$$

Again, the aim is to write Eq. (19) in terms of Eq. (21). In order to do this, we must first obtain the relation between the proper $n^{\mathrm{th}}$ order susceptibility tensor in terms of the improper one. Using Eq. (13) we can write the derivatives with respect to $\mathcal{E}'$ in

terms of derivatives with respect to $\mathcal{E}$:

$$
\begin{aligned}
\chi_{\mathcal{E}_1\ldots\mathcal{E}_n} &= \frac{\partial^{n-1}P'_{\mathcal{E}_1}}{\partial\mathcal{E}'_{\mathcal{E}_2}\ldots\partial\mathcal{E}'_{\mathcal{E}_n}} \\
&= \left[\prod_{i=2}^{n}(I+\tilde{\eta})^{-1}_{k_i\mathcal{E}_i}\right]\frac{\partial^{n-1}P'_{\mathcal{E}_1}}{\partial\mathcal{E}_{k_2}\ldots\partial\mathcal{E}_{k_n}} \\
&= \left[\prod_{i=1}^{n}(I+\tilde{\eta})^{-1}_{k_i\mathcal{E}_i}\right]\det(I+\tilde{\eta})\chi^{(\mathrm{i})}_{k_1\ldots k_n}
\end{aligned}
\tag{22}
$$

Expanding $\det(I+\tilde{\eta})$ and the products of $(I+\tilde{\eta})^{-1}$, and truncating to linear order, we get the following expression:

$$
\begin{aligned}
\chi_{\mathcal{E}_1\ldots\mathcal{E}_n} &= \left((1+\tilde{\eta}_{ii})\delta_{k_1\mathcal{E}_1}\ldots\delta_{k_n\mathcal{E}_n} - \sum_{i=1}^{n}\delta_{k_1\mathcal{E}_1}\ldots\underbrace{\tilde{\eta}_{k_i\mathcal{E}_i}}_{i^{\mathrm{th}}\text{position}}\ldots\delta_{k_n\mathcal{E}_n}\right)\chi^{(\mathrm{i})}_{k_1\ldots k_n} \\
&= (1+\tilde{\eta}_{ii})\chi^{(\mathrm{i})}_{\mathcal{E}_1\ldots\mathcal{E}_n} - \sum_{i=1}^{n}\chi^{(\mathrm{i})}_{\mathcal{E}_1\ldots k_i\ldots\mathcal{E}_n}\tilde{\eta}_{k_i\mathcal{E}_i}
\end{aligned}
.
\tag{23}
$$

Eq. (23) is the relation between $n^{\mathrm{th}}$ order susceptibility tensors in reduced and unreduced coordinates at finite strain. It is reassuring to see that when $\tilde{\eta}\to 0$ we have $\chi_{\mathcal{E}_1\ldots\mathcal{E}_n} = \chi^{(\mathrm{i})}_{\mathcal{E}_1\ldots\mathcal{E}_n}$, as expected. Obtaining the proper-improper relation for $A$ is now straightforward:

$$
\begin{aligned}
A_{\mathcal{E}_1\ldots\mathcal{E}_n\tilde{\eta}_1\tilde{\eta}_2} &= \frac{\partial}{\partial\tilde{\eta}_{\tilde{\eta}_1\tilde{\eta}_2}}\left((1+\tilde{\eta}_{ii})\chi^{(\mathrm{i})}_{\mathcal{E}_1\ldots\mathcal{E}_n} - \sum_{i=1}^{n}\chi^{(\mathrm{i})}_{\mathcal{E}_1\ldots k_i\ldots\mathcal{E}_n}\tilde{\eta}_{k_i\mathcal{E}_i}\right) \\
&= (1+\tilde{\eta}_{ii})\frac{\partial\chi^{(\mathrm{i})}_{\mathcal{E}_1\ldots\mathcal{E}_n}}{\partial\tilde{\eta}_{\tilde{\eta}_1\tilde{\eta}_2}} + \chi^{(\mathrm{i})}_{\mathcal{E}_1\ldots\mathcal{E}_n}\delta_{\tilde{\eta}_1\tilde{\eta}_2} - \sum_{i=1}^{n}\frac{\partial\chi^{(\mathrm{i})}_{\mathcal{E}_1\ldots k_i\ldots\mathcal{E}_n}}{\partial\tilde{\eta}_{\tilde{\eta}_1\tilde{\eta}_2}}\tilde{\eta}_{k_i\mathcal{E}_i} - \sum_{i=1}^{n}\chi^{(\mathrm{i})}_{\mathcal{E}_1\ldots k_i\ldots\mathcal{E}_n}\delta_{k_i\tilde{\eta}_1}\delta_{\mathcal{E}_i\tilde{\eta}_2}
\end{aligned}
.
\tag{24}
$$

Sending $\tilde{\eta}\to 0$, we get

$$
A_{\mathcal{E}_1\ldots\mathcal{E}_n\tilde{\eta}_1\tilde{\eta}_2} = A^{(\mathrm{i})}_{\mathcal{E}_1\ldots\mathcal{E}_n\tilde{\eta}_1\tilde{\eta}_2} + \delta_{\tilde{\eta}_1\tilde{\eta}_2}\chi_{\mathcal{E}_1\ldots\mathcal{E}_n} - \sum_{i=1}^{n}\chi_{\mathcal{E}_1\ldots\tilde{\eta}_1\ldots\mathcal{E}_n}\delta_{\tilde{\eta}_2\mathcal{E}_i}
\tag{25}
$$
